# Supplementary material for: Teachers Do More Than Teach: Compressing Image-to-Image Models
Source: arXiv:2103.03467 source file (2021-08-18)
Supplement: Supplementary file 1 [file fig_supp_cityscape.tex]

\begin{figure*}[]
\centering
\caption{
Additional results on Cityscapes dataset with Pix2pix model.
}
\label{fig:supp_city}
\end{figure*}
